# Supplementary material for: Asset Prices and Capital Share Risks: Theory and Evidence
Source: arXiv:2006.14023 source file (2020-06-24)
Supplement: Supplementary file 1 [file btvbsvcontrol.tex]

\subsubsubsection{B-TVB-SV Approach}
For robustness check, this paper also estimates the capital share factor with other control factors. According to previous estimates, the performances of capital share factor and other control factors are quite similar among all equity portfolios selected in this paper. Therefore, this section only estimate size/BM sorted portfolio returns.

This paper firstly plot the average break probabilities for each MFAPM including the capital share growth factor and a group of control factors. Break probabilities are estimated using 25 size/BM sorted portfolio returns. The first control factor group only includes consumption growth factor. Figure \ref{fig:breakkscons} plots the average break probabilities of factor loadings estimated by the 2-factor B-TVB-SV model which includes the capital share growth factor and the consumption growth factor. The time-average average break probabilities of capital share factor loadings are overall higher than those of the intersection or consumption growth factor loadings. The second group of control factors are Mkt, SMB and HML factors. Figure \ref{fig:breakksFF3} plots the average break probabilities of factor loadings estimated by the 4-factor B-TVB-SV model. Factors estimated are capital share factor, along with Fama-French 3 factors including Mkt, SMB and HML. The average break probabilities of capital share factor loadings are higher than those of Mkt, SMB and HML factor loadings for all portfolios, but are lower than that of the intersection.

With different control factors, the time-average break probabilities of capital share factor are of similar level as those derived by the parsimonious capital share factor model. The conclusion derived by the average break probabilities is inconsistent with the conclusion derived by the factor loadings spread approach by \cite{lettau2019capital}. Under F-MB bootstrap approach, the spread of capital share factor loading is low because that the MFAPM is estimated in a static manner within each simulation. The static approach omits the effect of time variation in volatilities. The distribution of capital share factor loading is narrower than control factors under the assumption of constant volatility, but wider than control factors under the assumption of stochastic volatility. %This finding further enhances the guess that risk factors \textcolor{red}{talk about this}
\begin{figure}[ht]
    \centering
    \includegraphics[width=\textwidth]{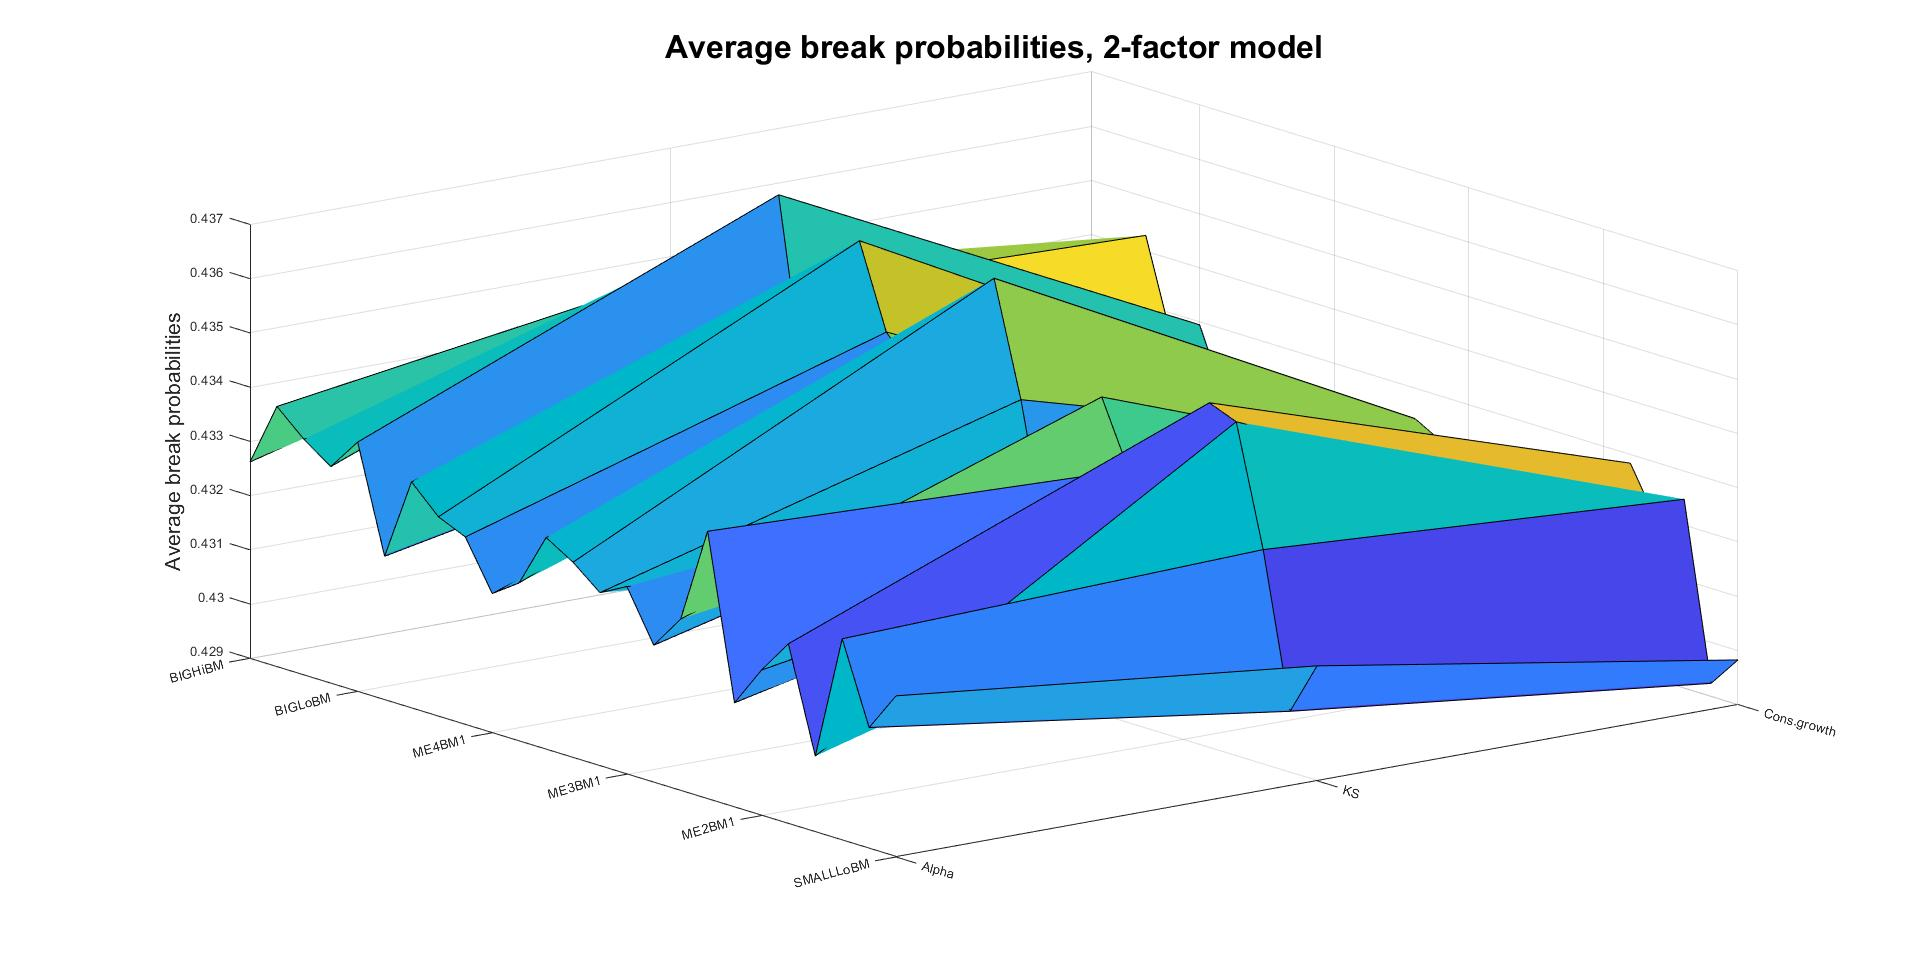}
    \caption{\textbf{B-TVB-SV average break probabilities of factor loadings.} Break probabilities are estimated using 25 size/BM sorted portfolio monthly returns. Factors estimated are the capital share factor with consumption growth factor. Sample spans 1964 January to 2018 August. The first 10-year data in the sample is used as training sample, and the sample estimated covers 1974 January to 2018 August.}
    \label{fig:breakkscons}
\end{figure}
\begin{figure}[ht]
    \centering
    \includegraphics[width=\textwidth]{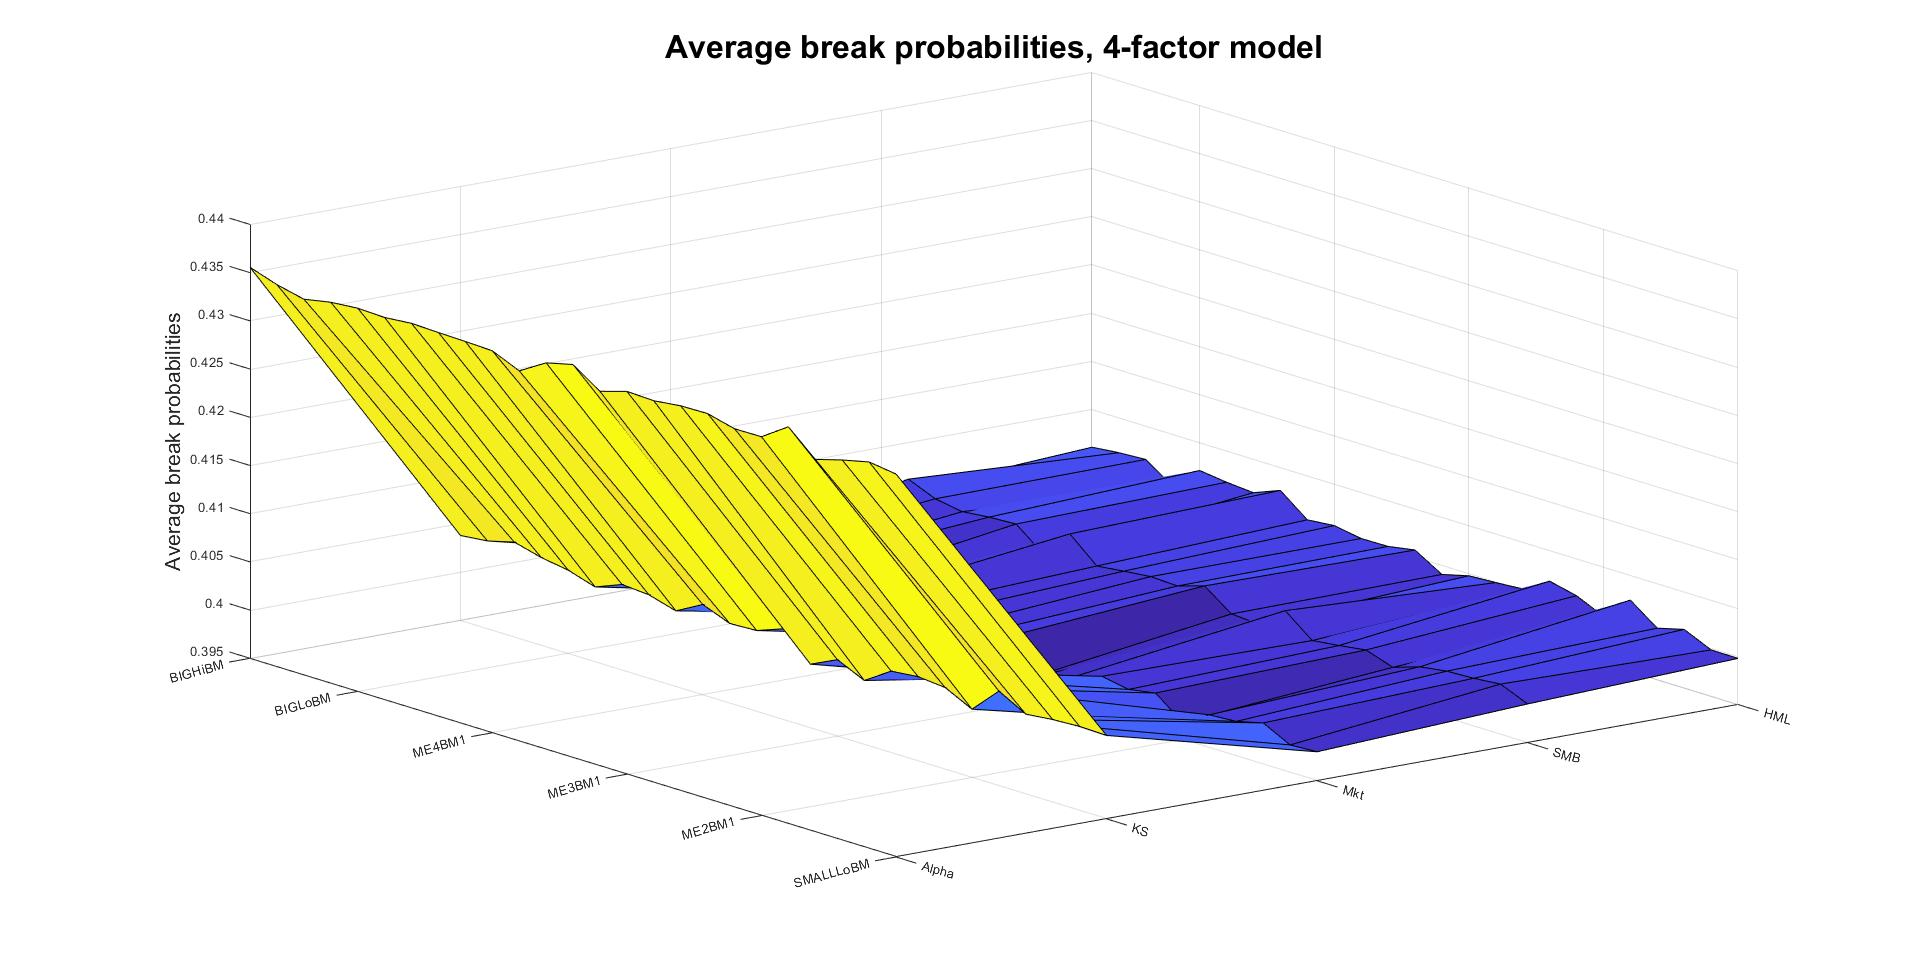}
    \caption{\textbf{B-TVB-SV average break probabilities of factor loadings.} Break probabilities are estimated using 25 size/BM sorted portfolio monthly returns. Factors estimated are the capital share factor with FF three factors including Mkt, SMB, and HML. Sample spans 1964 January to 2018 August. The first 10-year data in the sample is used as training sample, and the sample estimated covers 1974 January to 2018 August.}
    \label{fig:breakksFF3}
\end{figure}

Table \ref{tab:btvbsv_lambda_control} reports the risk premiums estimated using B-TVB-SV approach using size/BM sorted portfolio. Panel A and panel C reports the results obtained by the single consumption growth factor model and the 2-factor model including capital share factor and consumption growth factor. In panel A, the consumption growth risk premium is negative and significant. The sign is opposite as what is expected according to the static estimation from the previous sections. However, the sign of consumption growth risk premium is consistent with the rolling-window F-MB results, showing that the time variation of consumption growth factor loading affects the explanatory power of this factor dramatically. In panel C, the capital share risk premium is insignificant, which is similar as the results of the single capital share factor model. The significance of consumption risk premium decreases after adding the capital share factor into the MFAPM, but the consumption growth factor is still strong and has a significant risk premium. The width of the distribution of consumption growth factor is narrower compare to that in panel A. Panel B and panel D reports the results obtained by the FF 3-factor model and the 4-factor model including capital share factor and FF three factors. As shown by panel B and panel D, the HML risk premium is significant in both models while all other factors are insignificant. All risk premium distributions of the FF three factors are narrower in panel D than in panel C. Therefore, including capital share factor have similar impact on the risk premium distribution of the FF three factors as on the consumption growth factor. The significance of HML risk premium is not diminished by the capital share factor but increased after adding the capital share factor in the MFAPM. Therefore, the HML factor has a strong effect on levels of size/BM sorted portfolios in the sample estimated by this paper.

Keep the fact that the variance equation (equation (\ref{eq:sv})) might be misspecified, the risk premiums in Table \ref{tab:btvbsv_lambda_control} could be viewed as a indicator for identifying true factors which enters the mean equation (equation (\ref{eq:mfapm})). Commonly used MFAPMs simply pool all risk factors in the mean equation and ignore the potential effect of factors on the variance equation. Therefore, this paper proposes another view of MFAPM, which is identify the effect of risk factors before constructing the asset pricing model. In the case in this paper, without the effect of the serial correlation and common two-step problems, factors which enters the mean equation in the DGP of portfolio returns should has significant risk premiums under B-TVB-SV estimation; factors which have significant risk premiums under static F-MB estimation and related bootstrap estimation, but have insignificant risk premiums under B-TVB-SV estimation, should enters the variance equation for MFAPM. 
\begin{table}[h]
\centering
\caption{B-TVB-SV risk premium estimates.}
\begin{threeparttable}
\begin{tabular}{@{}lccccccc@{}}
\toprule\midrule
         & Average    & Std.err    & t-stat    & p-value    & 2.5\%    & 50\%   & 97.5\%   \\ \midrule
         & \multicolumn{7}{c}{Panel A: consumption growth factor model}\\
$\alpha$ & 1.208& 0.214&        5.648&        0.000&       -9.213&        1.475 &       9.612 \\
Cons.growth  & -0.838**&        0.272 &      -3.079 &       0.002 &      -13.46 &      -0.175 & 8.823 \\\midrule
         & \multicolumn{7}{c}{Panel B: FF 3-factor model}                          \\
$\alpha$ &  1.209**&    0.213&    5.676& 0.000&   -9.118&    1.467&    9.761          \\
Mkt      &  0.084&    0.551&    0.153&    0.879&  -15.508&   -0.060&   22.721          \\
SMB      &  0.848&    0.745&    1.139&    0.255&  -19.386&    0.186&   13.073         \\
HML      & -0.899*&    0.505&   -1.779&    0.076&  -15.641&   -0.161&   12.763      \\\midrule
         & \multicolumn{7}{c}{Panel C: 2-factor model}                          \\
$\alpha$ &  1.206**   &  0.213  & 5.665 & 0.000  &  -9.181& 1.492&9.581          \\
$F_{KS}$ &  0.073  & 0.218  &  0.334 &  0.739  & -8.439 & 0.090 & 9.867         \\
Cons.growth&  -0.687**  &  0.244 &  -2.812 &   0.005& -11.007& -0.098 & 8.228    \\\midrule
         & \multicolumn{7}{c}{Panel D: 4-factor model} \\
$\alpha$ &1.209**&	0.213&	5.672&	0.000&	-9.186&	1.467&	9.702\\
$F_{KS}$ &-0.044&	0.163&	-0.268&	0.789&	-6.088&	-0.006&	5.368\\
Mkt      &0.151&	0.502&	0.301&	0.763&	-15.232&	0.048&	20.334\\
SMB      &0.842&	0.688&	1.224&	0.222&	-13.665&	0.056&	11.469\\
HML      &-0.932**&	0.468&	-1.993&	0.047&	-12.888&	-0.190&	10.977\\ \bottomrule
\end{tabular}\\
\begin{tablenotes}
 Risk premiums in this table are estimated by a single capital share factor model using 25 size/BM sorted portfolios. Data used are monthly data from 1964 January to 2018 August. The first 10-year data are used as training sample for hyperparameter estimation, and the sample used for estimation spans 1974 January to 2018 August.
\end{tablenotes}
 \end{threeparttable}
     \label{tab:btvbsv_lambda_control}
\end{table}
%\newpage

%\newpage
