# Supplementary material for: Asset Prices and Capital Share Risks: Theory and Evidence
Source: arXiv:2006.14023 source file (2020-06-24)
Supplement: Supplementary file 2 [file control_bootstrap.tex]

\subsubsection{Static F-MB and F-MB Bootstrap}
This paper also estimates a single consumption growth factor model, and a 2-factor model including capital share factor and consumption growth factor. Table \ref{tab:static_lambdas_kscons} reports the static F-MB, F-MB bootstrap estimates and RM ratios. %In panel A, the risk premiums of consumption growth factor are positive but insignificant among all equity portfolios, and the $R^2$ estimates are all below 0.300, which are quite low compared to those estimated by capital share factor model.
In panel C, the 95\% bootstrap intervals of consumption growth risk premium all contain zero, and the lower bound of bootstrapped $R^2$ estimates are 0.000 of all portfolios. These results are in line with the well-known asset pricing puzzle: the consumption-based CAPM fails to explain portfolio returns (see \cite{lettau2001resurrecting}, \cite{parker2005consumption}, etc). Another explanation of the failure of consumption growth factor is about the measurement error effect: although the consumption growth factor is constructed using long-term growth (12-month growth rate), the time horizon is not long enough to cancel out the measurement error effect. As argued by \cite{parker2005consumption}, the 48-month consumption growth has higher pricing power than the 12-month consumption growth. Since this paper is not focused on testing the consumption growth factor, the insignificant results of the single consumption growth factor model is not a concern. 

Panel D in Table \ref{tab:static_lambdas_kscons} report bootstrap estimates of the 2-factor model. The risk premiums of capital share factor are significant among all portfolios under the F-MB bootstrap estimation. The bootstrapped $R^2$ hits zero at 5\% significance level for REV sorted portfolios. The signs of capital share risk premiums are still positive and their significant level are almost unaffected by the consumption growth factor. Meanwhile, the consumption growth factor remains insignificant among all portfolios. Compared to both the single capital share factor model and the single consumption growth factor model, the $R^2$ estimates are higher for the 2-factor model among all portfolios. Additionally, the 2-factor $R^2$ estimates approximate the sum of $R^2$ estimated by the two single factor model for each portfolio class. Assuming that canonical representative agent model holds, a strong positive correlation is expected to present between capital share growth and the consumption growth \cite{lettau2019capital}. However, the pattern of $R^2$ estimates is inconsistent with the expected collinearity between these two factors: the capital share factor could explain the variance which are consumption growth factor failed to explain, and the collinearity between these two factors is not very strong. Such pattern might be caused by the construction of capital share factor and consumption growth factor. However, in this paper, the capital share growth and consumption growth are both calculated over a 12 month period. Therefore, the construction of factors is consistent with the theoretical SDF specification in equation (\ref{eq:ks_apx}). Another explanation of such pattern comes from the theoretical base of the capital share factor: the agents are heterogeneous in the market due to the inequality of risk sharing and the concentration of wealth distribution \citep{lettau2019capital}. As shown by \cite{lettau2019capital}, when estimated using quarterly data, the pricing power of consumption growth factors constructed by various time horizons all decrease after including capital share factor. For monthly data, this paper focuses on testing the form of SDF in equation (\ref{eq:ks_apx}). Findings are consistent with the theoretical assumption that capital share is an additional component on top of consumption growth in CCAPM SDF \citep{lettau2019capital}. Additionally, for all portfolios, the pricing error represented by RM ratio is lower for capital share factor model than the single consumption growth factor model. Due to the fact that the consumption growth factor fails to explain return volatilities alone, the consumption growth factor seems to be less important than capital share factor in explaining variations of portfolio returns, and thus the majority of consumption risk is driven by inequality in the economy instead of the aggregate consumption. 
%\newpage
\begin{table}[ht]
\centering
\caption{Static F-MB and F-MB bootstrap risk premiums }

\begin{tabular}{@{}lcccc@{}}
\toprule
                    & Size/BM  & REV       & Size/INV       & Size/OP      \\ \midrule
                    & \multicolumn{4}{c}{Panel A: Static F-MB risk premiums}    \\
$\alpha$            	   &  0.974** & 0.828**   &    0.986**          &  1.519**            \\
                    & (0.000)   &  (0.000)      &  (0.000)           &  (0.000)            \\
Cons.growth          &  0.648  & 0.560       &  0.646             &   -0.966           \\
                        & (0.251) & (0.258)     &   (0.489)             &   (0.117)           \\
$R^2$                   &  0.055 & 0.287      &   0.044             &  0.124            \\ \midrule
                    & \multicolumn{4}{c}{Panel B: Static F-MB risk premiums}    \\
$\alpha$                &1.546**  &1.080**       & 1.507**          & 1.606**             \\
                    & (0.000)   & (0.000)     & (0.000)        & (0.000)      \\
$F_{KS}$               & 2.389**  & 0.826       & 2.024**        &2.054**         \\
                      & (0.013) & (0.443)     & (0.001)        &(0.017)      \\
Cons.growth             &-0.119  & 0.345      & -0.0856        & -0.444             \\
                      & (0.867) & (0.433)     & (0.944)        &(0.576)              \\
$R^2$                   & 0.557 & 0.311       & 0.631          &  0.810            \\ \midrule
                    & \multicolumn{4}{c}{Panel C: F-MB bootstrap risk premiums} \\
$\alpha$                 &0.972**  & 0.828**        & 0.989**          & 1.520**       \\
                     & [0.739, 1.193]& [0.633, 1.017] &[0.723, 1.250]&[1.282, 1.761]\\
Cons.growth          & 0.654& 0.562             &0.637           & -0.970       \\
                    &[-0.257, 1.571]& [-0.286, 1.361] &[-0.517, 1.769]& [-2.020, 0.055]\\
$\bar{R}^2$         &  0.091 &  0.201           &  0.055         &  0.131            \\
                    & [0.000, 0.391]& [0.000, 0.717] & [0.000, 0.320] & [0.000, 0.445]              \\
$\frac{RMSE}{RMSR}$  &  0.227& 0.148             &  0.218         &0.255         \\\midrule
                    & \multicolumn{4}{c}{Panel D: F-MB bootstrap risk premiums} \\
$\alpha$             &  1.545 & 1.078           &   1.509        & 1.605        \\
                    & [1.306, 1.783]& [0.465, 1.678]& [1.292,1.725]& [1.463, 1.739]\\
$F_{KS}$            &  2.385**& 0.821             &  2.028**         & 2.051**       \\
                    &[1.670, 3.098]& [-0.978, 2.642]& [1.480, 2.651] & [1.643, 2.484] \\
Cons.growth          &  -0.120& 0.350           &  -0.091        & -0.442       \\
                    &[-0.845, 0.559]& [-0.661,1.385]&[-0.895, 0.695]&[-0.973, 0.087] \\
$\bar{R}^2$         &  0.697& 0.259             & 0.735          &  0.844        \\
                    &[0.348, 0.905]& [0.000, 0.790]  & [0.405, 0.933]&[0.643,0.947]\\
$\frac{RMSE}{RMSR}$  & 0.158&  0.141                & 0.140           &  0.090       \\ 
\bottomrule
\end{tabular}
\\\begin{tablenotes}
The control factor in this table is the consumption growth factor. Portfolio returns used for estimation are REV, size/BM, size/INV, and size/OP sorted portfolios. Panel A reports static F-MB estimations of risk premiums of consumption growth factor. Panel B reports static F-MB estimations of risk premiums of capital share factor with consumption growth factor . Panel C reports F-MB bootstrap estimations of risk premiums of consumption growth factor. Panel D reports F-MB bootstrap estimations of risk premiums of capital share factor with consumption growth factor. All estimates are multiplied by 100. Static F-MB p-values are reported in brackets below estimates. Bootstrapped 95\% confidence intervals are reported in square brackets. ** denotes the estimate is significant at 5\% level. * denotes the estimate is significant at 10\% level. Sample spans the period 1974 January to 2018 August.
\end{tablenotes}
\label{tab:static_lambdas_kscons}
\end{table}
%\newpage
%\textcolor{red}{}
% Please add the following required packages to your document preamble:
% \usepackage{booktabs}
Additionally, this paper tests the FF 3-factor model and the 4-factor model including capital share growth factor and FF three factor, and the estimates are reported in Table \ref{tab:static_lambdas_ksff3}. Panel A and B report the static F-MB estimation of FF 3-factor model and 4-factor model respectively. In FF 3-factor model, the HML risk premium is significant when estimating size/INV and size/OP sorted portfolios. In the 4-factor model, the capital share risk premiums for size/BM and size/OP sorted portfolios are still positive and significant. Majority of FF three factor risk premiums in the 4-factor model are less significant than counterparts derived by the FF 3-factor model, but capital share factor does not affect the results for HML factor in size/INV sorted portfolio. Potential multicollinearities between the Mkt factor and the capital share factor present in these results. For example,  for size/INV sorted portfolio, the p-value of Mkt risk premium witnesses a large increase, while the $R^2$ is unchanged after adding capital share factor. Also, the p-values for Mkt risk premium is significantly attenuated by a larger extent compared to SMB or HML premiums. The correlation between Mkt factor and capital share factor fails within expectation. The assumption of capital share factor is based upon an stylised economy where the workers own no equity and only consume labor income, while the market participants, also investors, mainly consume the capital income gained from investment activities \citep{lettau2019capital}. Therefore, the aggregate behavior of the equity market should be highly correlated if this assumption hold. In general, the FF 3-factor model explains the variation of returns well, with high estimated $R^2$ for all equity portfolios. Most of $R^2$ estimates derived by the FF 3-factor are of similar magnitude with the $R^2$ estimates for the single capital share factor model, which is quite similar with results derived by \cite{lettau2019capital} using quarterly data. In quarterly data, the parsimonious capital share factor model explains a larger fraction of expected returns on equity portfolios than does the FF 3-factor model \cite{lettau2019capital}. However, in monthly data estimated by this paper, the FF three factors and capital share factor show an opposite pattern: the performance for FF three factors are more stable than capital share factor, as indicated by a generally higher $R^2$ estimated by all equity portfolios. Panel C and panel D compares the bootstrap estimates of the FF 3-factor and the 4-factor model. The bootstrap means of estimates are about the same as the counterparts estimated by static F-MB approach. For all portfolios, the pricing error represented by RM ratio is lower for FF 3-factor model  compared to the single capital share factor model, which is also inconsistent with the conclusion derived by \cite{lettau2019capital}. The F-MB bootstrap results are reported in panel C and panel D. The bootstrap procedure corrects the firm effect of portfolio returns, and the risk premiums of the FF three factors are more significant compared to under static F-MB estimation. In general, the bootstrap results are similar as the static results: capital share risk premium is significant , and the explanatory power of all FF three factors is diminished among most portfolios. Only for size/INV sorted portfolio returns, capital share factor is dominated by the Mkt factor and the HML factor.

%\newpage
\begin{table}[H]
\centering
\caption{Static F-MB and F-MB bootstrap risk premiums.} 
\begin{threeparttable}

\begin{tabular}{@{}lcccc@{}}
\toprule
                    & Size/BM & REV             & Size/INV       & Size/OP      \\ \midrule
                    & \multicolumn{4}{c}{Panel A: Static F-MB risk premiums}    \\
$\alpha$             &1.090**&1.031**  & 1.157** & 1.107**      \\
                    & (0.000)&(0.000) & (0.000)& (0.000)           \\
Mkt                  &0.976 & -1.654  & 0.809  & 0.957\\
                    & (0.332)& (0.473)& (0.495)& (0.440)    \\
SMB                 &-0.607 & -1.459  & 0.221  &0.214  \\
                    &(0.308)&(0.223)  & (0.742)&(0.767)     \\
HML                  &1.345*& -2.324   &2.786**  &3.109**\\
                    &(0.066)& (0.287) &(0.011) & (0.016)      \\
$R^2$               &0.576& 0.463     & 0.819  & 0.713 \\ \midrule
                    & \multicolumn{4}{c}{Panel B: Static F-MB risk premiums}    \\
$\alpha$            &1.375**&1.394**    &1.171**& 1.492**\\
                    & (0.003)&(0.000) & (0.000)& (0.000)                 \\
$F_{KS}$            &1.489**& 1.266    &0.205&1.958**\\
                    & (0.022)&(0.406)&(0.794)&(0.021)           \\
Mkt                 &-0.032&-2.126   &0.756& -0.667 \\
                    & (0.976)& (0.337)&(0.548)&(0.571)                    \\
SMB                 &-0.587&-1.624   &0.213& -0.057\\
                    &(0.351)&(0.173) &(0.740)&(0.927)               \\
HML                 &  0.908&-1.162  &2.722**& 1.308  \\
                    & (0.220)&(0.409) &(0.003)&(0.133)      \\
$R^2$               &0.647& 0.534    & 0.819  &0.846 \\ \midrule
                    & \multicolumn{4}{c}{Panel C: F-MB bootstrap risk premiums} \\
$\alpha$            &1.091**& 1.032**   &  1.157** & 1.106**  \\
                    &[0.941, 1.241]& [0.749, 1.311]&[1.066, 1.244]&[0.977, 1.234] \\
Mkt                 &0.976**& -1.651  & 0.808**  & 0.954** \\
                    &[0.047, 1.931]& [-4.395, 1.104]&[0.257, 1.334]&[0.221, 0.695]      \\
SMB                 & -0.613& -1.459& 0.219  & 0.213   \\
                    &[-1.375, 0.158]&[-3.345, 0.419]&[-0.247, 0.719]&[-0.424, 0.844]\\
HML                 & 1.343**& -2.334** & 2.780**  & 3.016**    \\
                    &[0.605, 2.056]&[-4.204, -0.465]&[2.158, 3.416]& [2.006, 3.959] \\
$\bar{R}^2$          &0.646& 0.697  & 0.858  &0.763    \\
                    &[0.330, 0.860]&[0.090, 0.960]&[0.662, 0.958]&[0.461, 0.926]     \\
$\frac{RMSE}{RMSR}$ &0.105& 0.092&0.064&0.094   \\\midrule
                    & \multicolumn{4}{c}{Panel D: F-MB bootstrap risk premiums} \\
$\alpha$            &1.377**&1.392**   &1.171**& 1.493**\\
                    &[1.088, 1.665]&[0.716, 2.058]&[0.996, 1.337]&[1.307, 1.673]\\
$F_{KS}$             &1.490**& 1.257 &0.208&    1.962**\\
                    &[0.519, 2.465]&[-0.733, 3.217]&[-0.378, 0.815]&[1.386, 2.521] \\
Mkt                 & -0.034&-2.130  &0.752**&   -0.672\\
                    &[-1.156, 1.07]&[-5.068, 0.828]&[0.029, 1.467]& [-1.409, 0.060]\\
SMB                 & -0.594& -1.617 &0.210&   -0.060\\
                    &[-1.356, 0.168]&[-3.604, 0.429]&[-0.276, 0.724]&[-0.553, 0.444]\\
HML                 & 0.908**&-1.169  &2.713** &    1.306**\\
                    &[0.152, 1.660]& [-3.212, 0.836]&[1.970, 3.494]&[0.491, 2.124] \\
$\bar{R}^2$         &0.723& 0.693&0.860&0.871     \\
                    &[0.428, 0.899]&[0.058, 0964]&[0.666, 0.958]&[0.7072, 0.955]     \\
$\frac{RMSE}{RMSR}$ &0.063&0.109&0.077&0.116  \\
\bottomrule
\end{tabular}
\\
\begin{tablenotes}
The control factors are the FF three factors including Mkt, SMB, and HML. Portfolio returns are REV, size/BM, size/INV, and size/OP sorted portfolios. Panel A reports static F-MB estimations of risk premiums of FF three factors. Panel B reports static F-MB estimations of risk premiums of capital share factor with FF three factors. Panel C reports F-MB bootstrap estimations of risk premiums of FF three factors. Panel D reports F-MB bootstrap estimations of risk premiums of captial share growth factor with FF three factors. All estimates are multiplied by 100. P-values are reported in brackets below estimates. Bootstrapped 95\% confidence intervals are reported in square brackets. ** denotes the estimate is significant at 5\% level. * denotes the estimate is significant at 10\% level. Sample spans the period 1974 January to 2018 August.
\end{tablenotes}
\end{threeparttable}
\label{tab:static_lambdas_ksff3}
\end{table}
