# Supplementary material for: Asset Prices and Capital Share Risks: Theory and Evidence
Source: arXiv:2006.14023 source file (2020-06-24)
Supplement: Supplementary file 3 [file rollingwindow.tex]

\subsubsection{Rolling-window Regression}
\begin{table}[H]
\centering
\caption{Rolling-window F-MB risk premiums}

\begin{tabular}{@{}lcccc@{}}
\toprule
&\multicolumn{4}{c}{Rolling-window F-MB risk premiums}\\\midrule
                    & Size/BM& REV                            & Size/INV & Size/OP            \\\midrule
                    & \multicolumn{4}{c}{Panel A: consumption growth factor model}\\
$\alpha$            &1.099**& 0.953**& 1.142**&1.054**\\
                    &(0.000)&(0.000)&(0.000)& (0.000)\\
Cons.growth         &-0.096&0.074&-0.132*&-0.076 \\
                    &(0.151)&(0.406)&(0.051)&(0.246)\\
$R^2$               &0.195&0.494&0.131& 0.030\\ \midrule
                    & \multicolumn{4}{c}{Panel B: FF 3-factor model}\\
$\alpha$            &1.111**& 0.907**&1.086**&1.026**\\
                    & (0.000)&(0.000)&(0.000)&(0.000)\\
Mkt                 &0.162& -0.211&0.353&0.351\\
                    &(0.533)& (0.514)&(0.145)&(0.159)\\
SMB                 &-0.230& 0.087&-0.279*&-0.030\\
                    &(0.144)& (0.728)&(0.068)&(0.838)\\
HML                 &0.004& 0.177&0.046&-0.139\\
                    &(0.980)& (0.448)&(0.779)&(0.402)\\
$R^2$               &0.559&0.746&0.592& 0.413\\ \midrule
                    & \multicolumn{4}{c}{Panel C: 2-factor model}  \\
$\alpha$            &1.006**& 0.778**&1.013**&0.929**\\
                    & (0.000)&(0.000)&(0.000)&(0.000)\\
$F_{KS}$            &-0.028& 0.035&0.083&0.059\\
                    &(0.758)& (0.739)&(0.378)&(0.520)\\
Cons.growth         &-0.091& -0.021&-0.160**&-0.122*\\
                    &(0.160)& (0.809)&(0.013)&(0.054)\\
$R^2$               &0.400& 0.647&0.381&0.402\\ \midrule                   
                    & \multicolumn{4}{c}{Panel D: 4-factor model}\\
$\alpha$            &1.175**& 0.724**&1.082**&1.052**\\
                    &(0.000)& (0.004)&(0.000)&(0.000)\\
$F_{KS}$            &-0.029& -0.023&0.036&0.080\\
                    &(0.734)& (0.836)&(0.663)&(0.330)\\
Mkt                 &0.059& -0.410&0.178&0.261\\
                    &(0.803)& (0.216)&(0.435)&(0.276)\\
SMB                 &-0.169& 0.176&-0.253*&-0.055\\
                    &(0.231)& (0.484)&(0.080)&(0.691)\\
HML                 &0.122& 0.247&0.069&-0.062\\
                    &(0.447)& (0.272)&(0.659)&(0.696)\\
$R^2$               &0.635& 0.860&0.599&0.658\\ \bottomrule
\end{tabular}
\\
\begin{tablenotes}
The control factors are 1) the consumption growth factor and 2) FF three factors including Mkt, SMB, and HML. Portfolio returns used for estimation are REV, size/BM, size/INV, and size/OP sorted portfolios. Panel A reports risk premiums of consumption growth factor. Panel B reports risk premiums of the consumption growth factor.  Panel C reports risk premiums of the FF three factors.  Panel D reports risk premiums of the capital share growth factor with consumption growth factor as control factor. Panel E reports risk premiums of the capital share growth factor with FF three factors as control factors. All estimates are multiplied by 100. P-values are reported in brackets below estimates. ** denotes the estimate is significant at 5\% level. * denotes the estimate is significant at 10\% level. Sample spans the period 1974 January to 2018 August.
\end{tablenotes}
\label{tab:rw_lambdas_all}
\end{table}
