# Supplementary material for: Asset Prices and Capital Share Risks: Theory and Evidence
Source: arXiv:2006.14023 source file (2020-06-24)
Supplement: Supplementary file 4 [file converge.tex]

\subsection{MCMC Convergence Analysis}

\begin{table}[H]
\centering
\begin{tabular}{@{}lccc@{}}
\toprule\midrule
\multicolumn{4}{c}{Summary of Convergence Diagnostics}                     \\ \midrule
                   & Parameters & 5\% Rejection Rate & 10\% Rejection Rate \\
$B$                & 24840      & 0.0102             & 0.0347              \\
$K_\beta,K_\sigma$ & 33120      & 0.0133             & 0.0400              \\
$\Sigma$           & 8280       & 0.0108             & 0.0317              \\
$Q$                & 115        & 0.0000             & 0.0000              \\
$\pi$              & 115        & 0.0000             & 0.0000              \\ \bottomrule
\end{tabular}
\end{table}
 \subsection{Likelihood Function}
The complete likelihood function, namely joint density of the data and state variables in equation (\ref{eq:btvbsv1}) and equation (\ref{eq:btvbsv2}) is as follows:
\begin{align}
    &p(R,B,K,\Sigma \mid \lambda,\theta,F)\nonumber\\
    &=\prod^T_{t=1}\bigg( \prod^N_{i=1}p(r_{it} \mid \lambda_t,F_t,\beta_{i,t},\beta_{i,t-1},\sigma^2_{i,t} ) \nonumber\\
    &\times p(\sigma^2_{i,t}\mid \sigma^2_{i,t-1},\kappa_{i\upsilon,t},q^2_{i\upsilon})\pi^{\kappa_{i\upsilon,t}}_{i\upsilon}(1-\pi_{i\upsilon})^{1-\kappa_{i\upsilon,t}} \nonumber\\
    &\times \Big( \prod^K_{j=0} p(\beta^2_{ij,t}\mid \sigma^2_{ij,t-1},\kappa_{ij,t},q^2_{ij})\pi^{\kappa_{ij,t}}_{ij}(1-\pi_{ij})^{1-\kappa_{ij,t}} \Big) \bigg)
\end{align}
where $K=(K_\beta,K_\sigma)$. Therefore, the posterior density is written as $p(\theta,B,K,\Sigma,\lambda \mid R, F)\propto p(\theta, \lambda)p(R,B,K,\Sigma \mid \lambda, \theta,F)$. The sampling process of posteriors follows \cite{bianchi2017macroeconomic}.
