# Supplementary material for: Asset Prices and Capital Share Risks: Theory and Evidence
Source: arXiv:2006.14023 source file (2020-06-24)
Supplement: Supplementary file 5 [file garch.tex]

\subsection{Sanity Check Regression}
\begin{table}[ht]
\centering

\begin{tabular}{@{}lcccccc@{}}
\toprule\midrule
            & Intersection & $ln(\sigma^2_{t-1})$ & $F_{KS}$ \\\midrule
SMALLLoBM & 2.325**       & 0.081**           & 6.972* \\
            & (0.000)       & 0.039*    & (0.079)   \\
ME1BM2    & 2.280**       & (0.054)      & 6.644**   \\
            & (0.000)       & (0.167)    & (0.049)   \\
ME1BM3    & 1.852**       & 0.102**    & 9.729**  \\ 
            & (0.000)       & (0.009)     & (0.006)   \\
ME1BM4    & 1.747**      & 0.052   & 5.423  \\ 
            & (0.000)       & (0.181)        & (0.155)   \\
SMALLHiBM & 1.757**       & 0.064    & 10.395** \\
            & (0.000)       & (0.103)    & (0.009)   \\
ME2BM1    & 2.212**       & 0.072*     & 8.334** \\  
             & (0.000)       & (0.064)     & (0.028)   \\
ME2BM2    & 2.010**       & 0.045      & 8.623** \\ 
            & (0.000)       & (0.253)      & (0.015)   \\
ME2BM3    & 1.800*       & 0.0110       & 7.290** \\  
            & (0.000)      & (0.778)        & (0.048)   \\
ME2BM4    & 1.677**       & 0.066**       & 5.308 \\ 
            &(0.000)       & (0.092)      & (0.151)   \\
ME2BM5    & 1.905**       & 0.068*          & 4.996  \\
            &(0.000)       & (0.083)     & (0.174)   \\
ME3BM1    & 2.144**       & 0.102**       & 9.414** \\  
            & (0.000)       & (0.009)       & (0.005)   \\
ME3BM2    & 1.815**       & 0.054        & 5.800* \\  
            & (0.000)       & (0.166)       & (0.095)   \\
ME3BM3    & 1.613**       & 0.027*          & 7.554* \\ 
            & (0.000)       & (0.493)     & (0.063)   \\
ME3BM4    & 1.433**      & 0.099**      & 5.828  \\ 
            & (0.000)       & (0.012)     & (0.122)   \\
ME3BM5    & 1.614**       & 0.1182    & 4.764  \\ 
            & (0.000)       & (0.003)    & (0.204)   \\
ME4BM1    & 1.889**       & 0.075*      & 4.290 \\  
            &(0.000)       & (0.056)     & (0.252)   \\
ME4BM2    & 1.607**       & 0.077**     & 5.085  \\ 
            & (0.000)       & (0.048)     & (0.158)   \\
ME4BM3    & 1.486**       & 0.070*     & 5.925  \\ 
            & (0.000)       & (0.072)   & (0.114)   \\
ME4BM4    & 1.346**       & 0.126      & 8.162** \\ 
            &(0.000)      & (0.001)    & (0.038)   \\
ME4BM5    & 1.846**       & 0.0374      & 7.614** \\ 
            & (0.000)       & (0.341)        & (0.041)   \\
BIGLoBM   & 1.481**       & 0.030   & 5.645 \\  
            & (0.000)       & (0.449)   & (0.134)   \\
ME5BM2    & 1.375**       & 0.0369    & 2.397 \\ 
            &(0.000)       & (0.346)          & (0.523)   \\
ME5BM3    & 1.282**       & 0.082**   & 5.024  \\
            & (0.000)      & (0.035)     & (0.154)   \\
ME5BM4    & 1.473**       & 0.003     & 8.778**  \\
            &(0.000)       & (0.947)       & (0.017)   \\
BIGHiBM   & 1.683**      & 0.028     & 9.521**  \\ 
            & (0.000)       & (0.481)        & (0.020)   \\ \bottomrule\\
\end{tabular}
\caption{Sanity check regression of (G)ARCH effect of the capital share factor.}
\label{rab:garch_check}
\end{table}
\newpage
