# Supplementary material for: Asset Prices and Capital Share Risks: Theory and Evidence
Source: arXiv:2006.14023 source file (2020-06-24)
Supplement: Supplementary file 6 [file hyper.tex]

\subsection{Hyperparameter Selection}
Prior hyperparameters for B-TVB-SV in this paper are identical to \cite{bianchi2017macroeconomic} as shown in Table \ref{tab:hyperparameter}:
\begin{table}[H]
\centering
\begin{tabular}{@{}lcccc@{}}
\toprule\midrule
Variables   &Parameter             & Values & Parameter            & Values \\ \midrule
$\beta_{ij}$ & $\mu_\beta$                 &$\beta_{OLS}$  &$\sigma^2_\beta$    &$\sigma^2_{OLS}$\\
$ln(\sigma^2_{i})$ & $\mu_{ln(\sigma^2)}$                 &2 &$\sigma^2_{ln(\sigma^2)}$   &10\\
$\kappa_{ij}$ &$a_{ij}$              & 3.2    &$b_{ij}$              & 60      \\
$\kappa_{i\upsilon}$& $a_{i\upsilon}$      & 1     & $b_{i\upsilon}$      & 99     \\
$q_{ij}$&$\gamma_{ij}$         & 0.5    &$\theta_{ij}$         & 100    \\
$q_{i\upsilon}$& $\gamma_{i\upsilon}$ & 0.2    & $\theta_{i\upsilon}$ & 50     \\
$\lambda$&$\underline{\lambda}$ & 0      &$\underline{V}$       & 1000    \\
$\tau^2$  & $\psi_0$             & 0.1   & $\Psi_0$             & 10     \\ \bottomrule\\
\end{tabular}
\caption{B-TVB-SV: prior hyperparameters. OLS denotes the OLS estimation obtained by the first 10-year training sample}
\label{tab:hyperparameter}
\end{table}
