# Supplementary material for: Asset Prices and Capital Share Risks: Theory and Evidence
Source: arXiv:2006.14023 source file (2020-06-24)
Supplement: Supplementary file 7 [file notes.tex]

\begin{table}[ht]
\centering
\begin{tabular}{@{}lcccc@{}}
\toprule \midrule
Portfolio/Factor   & \multicolumn{1}{l}{Mean} & \multicolumn{1}{l}{Median} & \multicolumn{1}{l}{Std.dev.} & \multicolumn{1}{l}{Sharpe ratio} \\ \midrule
&  \multicolumn{4}{c}{10 industry portfolios, value-weighted}                                                                                   \\ 
Nondurable goods   & 1.107                    & 1.135                      & 4.466                        & 0.248                            \\
Durable goods      & 0.809                    & 0.815                      & 6.657                        & 0.121                            \\
Manufacturing      & 0.988                    & 1.195                      & 5.207                        & 0.190                            \\
Energy             & 1.163                    & 0.990                       & 5.677                        & 0.205                            \\
High-tech          & 0.924                    & 0.950                       & 6.907                        & 0.134                            \\
Telecommunications & 0.948                    & 1.175                      & 4.880                        & 0.194                            \\
Shops and retail   & 0.974                    & 1.060                       & 5.448                        & 0.179                            \\
Healthcare         & 0.990                    & 1.050                       & 5.085                        & 0.195                            \\
Utilities          & 0.933                    & 0.995                      & 4.134                        & 0.226                            \\
Other              & 0.871                    & 1.320                       & 5.435                        & 0.160                            \\ \midrule
&  \multicolumn{4}{c}{10 Size-sorted portfolios, value-weighted}                                                                                \\
Decile 1           & 1.073                    & 1.205                      & 6.362                        & 0.169                            \\
Decile 2           & 1.083                    & 1.390                       & 6.497                        & 0.167                            \\
Decile 3           & 1.125                    & 1.545                      & 6.170                        & 0.182                            \\
Decile 4           & 1.089                    & 1.500                        & 5.957                        & 0.183                            \\
Decile 5           & 1.127                    & 1.680                       & 5.816                        & 0.194                            \\
Decile 6           & 1.081                    & 1.180                       & 5.421                        & 0.199                            \\
Decile 7           & 1.088                    & 1.255                      & 5.389                        & 0.202                            \\
Decile 8           & 1.024                    & 1.275                      & 5.267                        & 0.195                            \\
Decile 9           & 0.986                    & 1.335                      & 4.857                        & 0.203                            \\
Decile 10          & 0.844                    & 1.075                      & 4.473                        & 0.189                            \\ \midrule
&   \multicolumn{4}{c}{Bond returns}                                                                                                             \\
10-year T-note     & 0.679                    & 0.628                      & 2.289                        & 0.297                            \\
15-year T-note     & 0.635                    & 0.585                      & 1.611                        & 0.394                            \\
Baa Crop. bond     & 0.831                    & 0.863                      & 3.253                        & 0.255  \\
~~~~(10-20 years)     &                    &                     &                      &                        
\end{tabular}

\caption{Descriptive statistics: portfolio returns \citep{bianchi2017macroeconomic}. Portfolio returns are categorised into three groups: returns of 10 value-weighted industry portfolios, returns of 10 value-weighted size-sorted portfolios and returns of three bond returns. Data are monthly and covers the sample period 1972:01$-$2011:12.}
\label{tab:summary}
\end{table}
